# Supplementary material for: Synthesizing Abstract Transformers
Source: arXiv:2105.00493 source file (2022-08-15)
Supplement: Supplementary file 1 [file appendix.tex]

\section{Appendix}
\label{App:appendix}

\subsection{String Abstract Domains}
\label{App:StringAbstractDomains}

%\subsubsection{Sketch of $\abst{concat}{}$ in the $\mathcal{SH}$ abstract domain}
%\label{App:stringHashDsltemplate}
%\figref{concatSk} shows the sketch that we used to synthesize the
%abstract transformer for the \texttt{concat} function.
%Among the options specified within \texttt{\{...|...|...|...\}},
%the Sketch synthesizer selects an option that makes the resulting program
%consistent with the specification.
%For example, at \lineref{HashDSLChoice}, Sketch selects from among
%the provided \texttt{rotateLeft(r,1)} and \texttt{rotateRight(r,1)} options.

\subsubsection{Plots of the performance and precision of synthesized transformers}
\figrefs{COvaluation}{CoPsEvaluation} show the performance and precision of the synthesized transformers in the $\csdom$ and $\csdom \times \psdom$ domains, respectively.

%\skmchanged{
\subsubsection{Detailed Results}
A detailed log of our experiments on synthesizing abstract transformers for abstract string
domains is given in \tableref{StringDomLogicalLog}.
The table headers should be interpreted as follows:
\begin{itemize}
\item \textbf{Domain}: Domain name
\item $\mathbf{f}$: Concrete function name
\item \textbf{\#SO}: Number of times a soundness query is performed
\item \textbf{\#PO}: Number of times a precision query is performed
\item \textbf{\#PosEx}: Number of positive examples 
\item \textbf{\#NegEx}: Number of negative examples 
\item \textbf{\#MaxSat}: Number of times \textsc{MaxSatSynthesis} is invoked
\item \textbf{\#Dropped}: Total number of examples dropped during \textsc{MaxSatSynthesis}
\item \textbf{SO Time (s)}: Total time taken in seconds by soundness queries
\item \textbf{PO Time (s)}: Total time taken in seconds by precision queries
\item \textbf{Time (s)}: Total time taken in seconds
\end{itemize}

%\begin{figure}[b]
%	\lstinputlisting[numbers=left]{./code/hashDSLSketch.sk}
%	\caption{Sketch to synthesize abstract transformer for $\mathtt{concat}^\sharp$ in $\mathcal{SH}$\label{Fi:concatSk}}
%\end{figure}

\begin{figure}[b]
	\centering
	\includegraphics[scale=0.35]{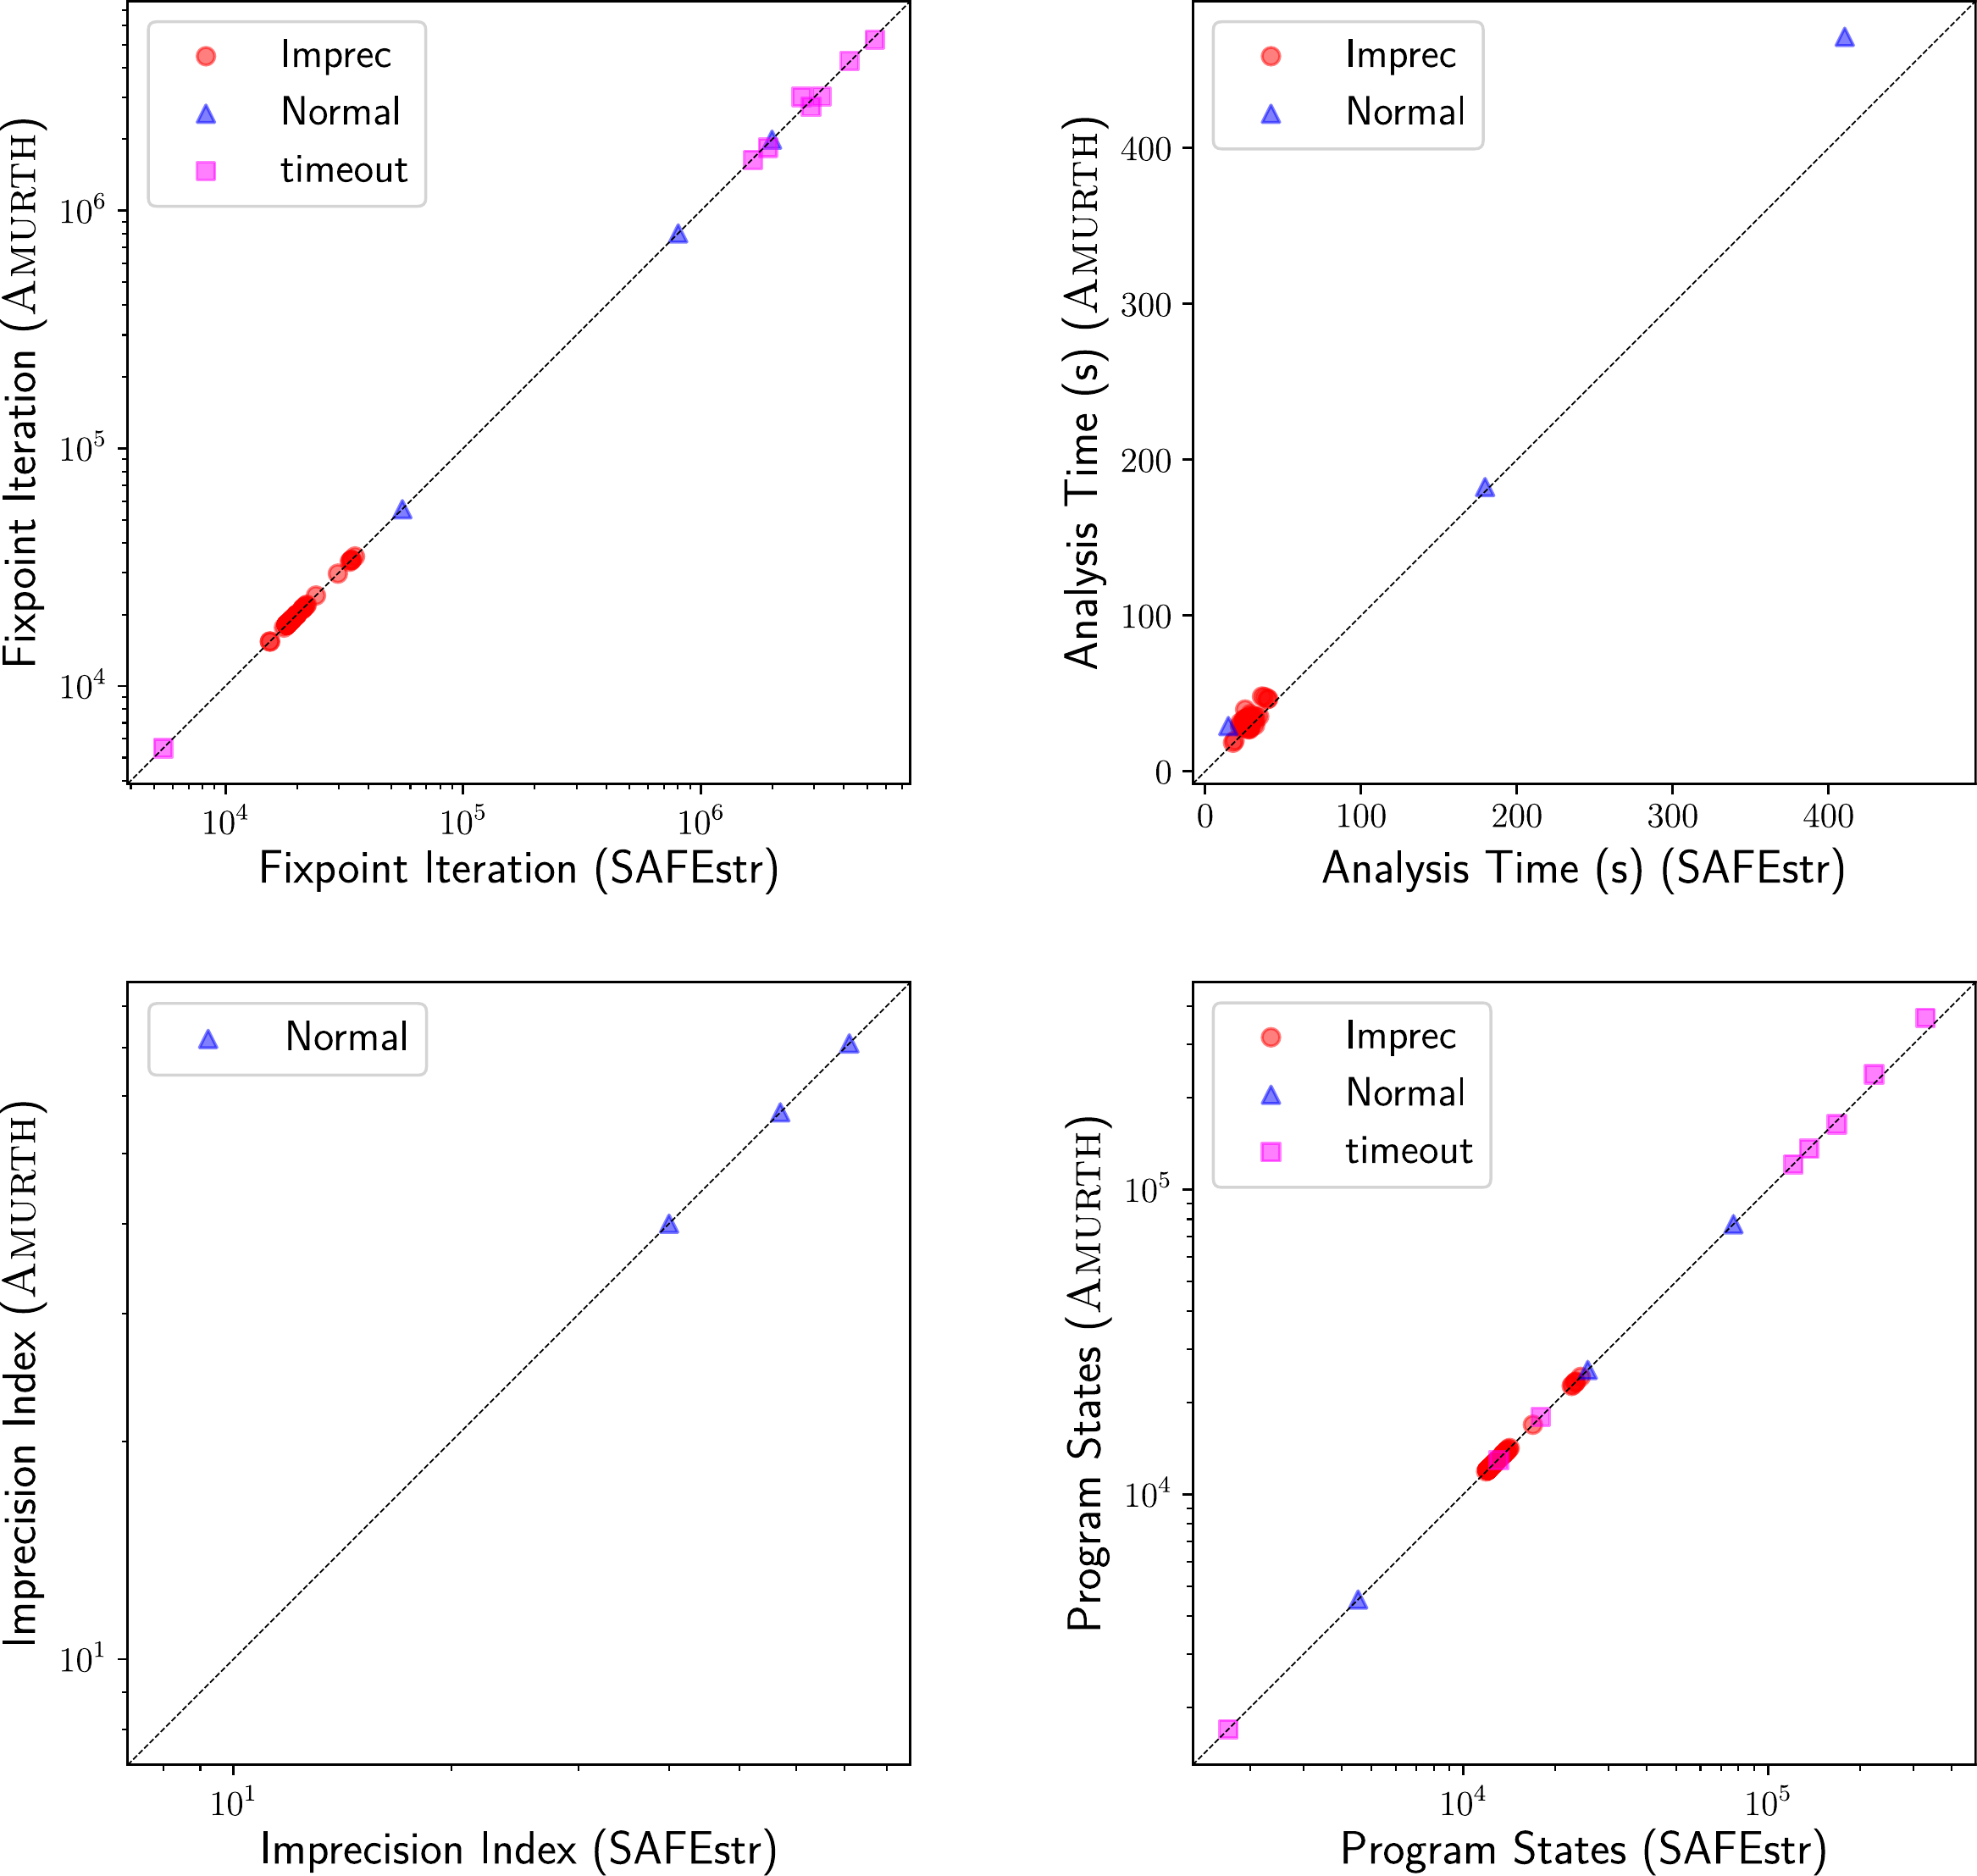}
	\caption{Performance and precision of the synthesized transformers with the $\csdom$ domain.
		(\nsquare{magenta}~: timeout; \ntriangle{blue}~: normal termination; \ncircle{red}~: termination due to imprecision trigger)
		\label{Fi:COvaluation}}
\end{figure}

\begin{figure}
	\centering
	\includegraphics[scale=0.35]{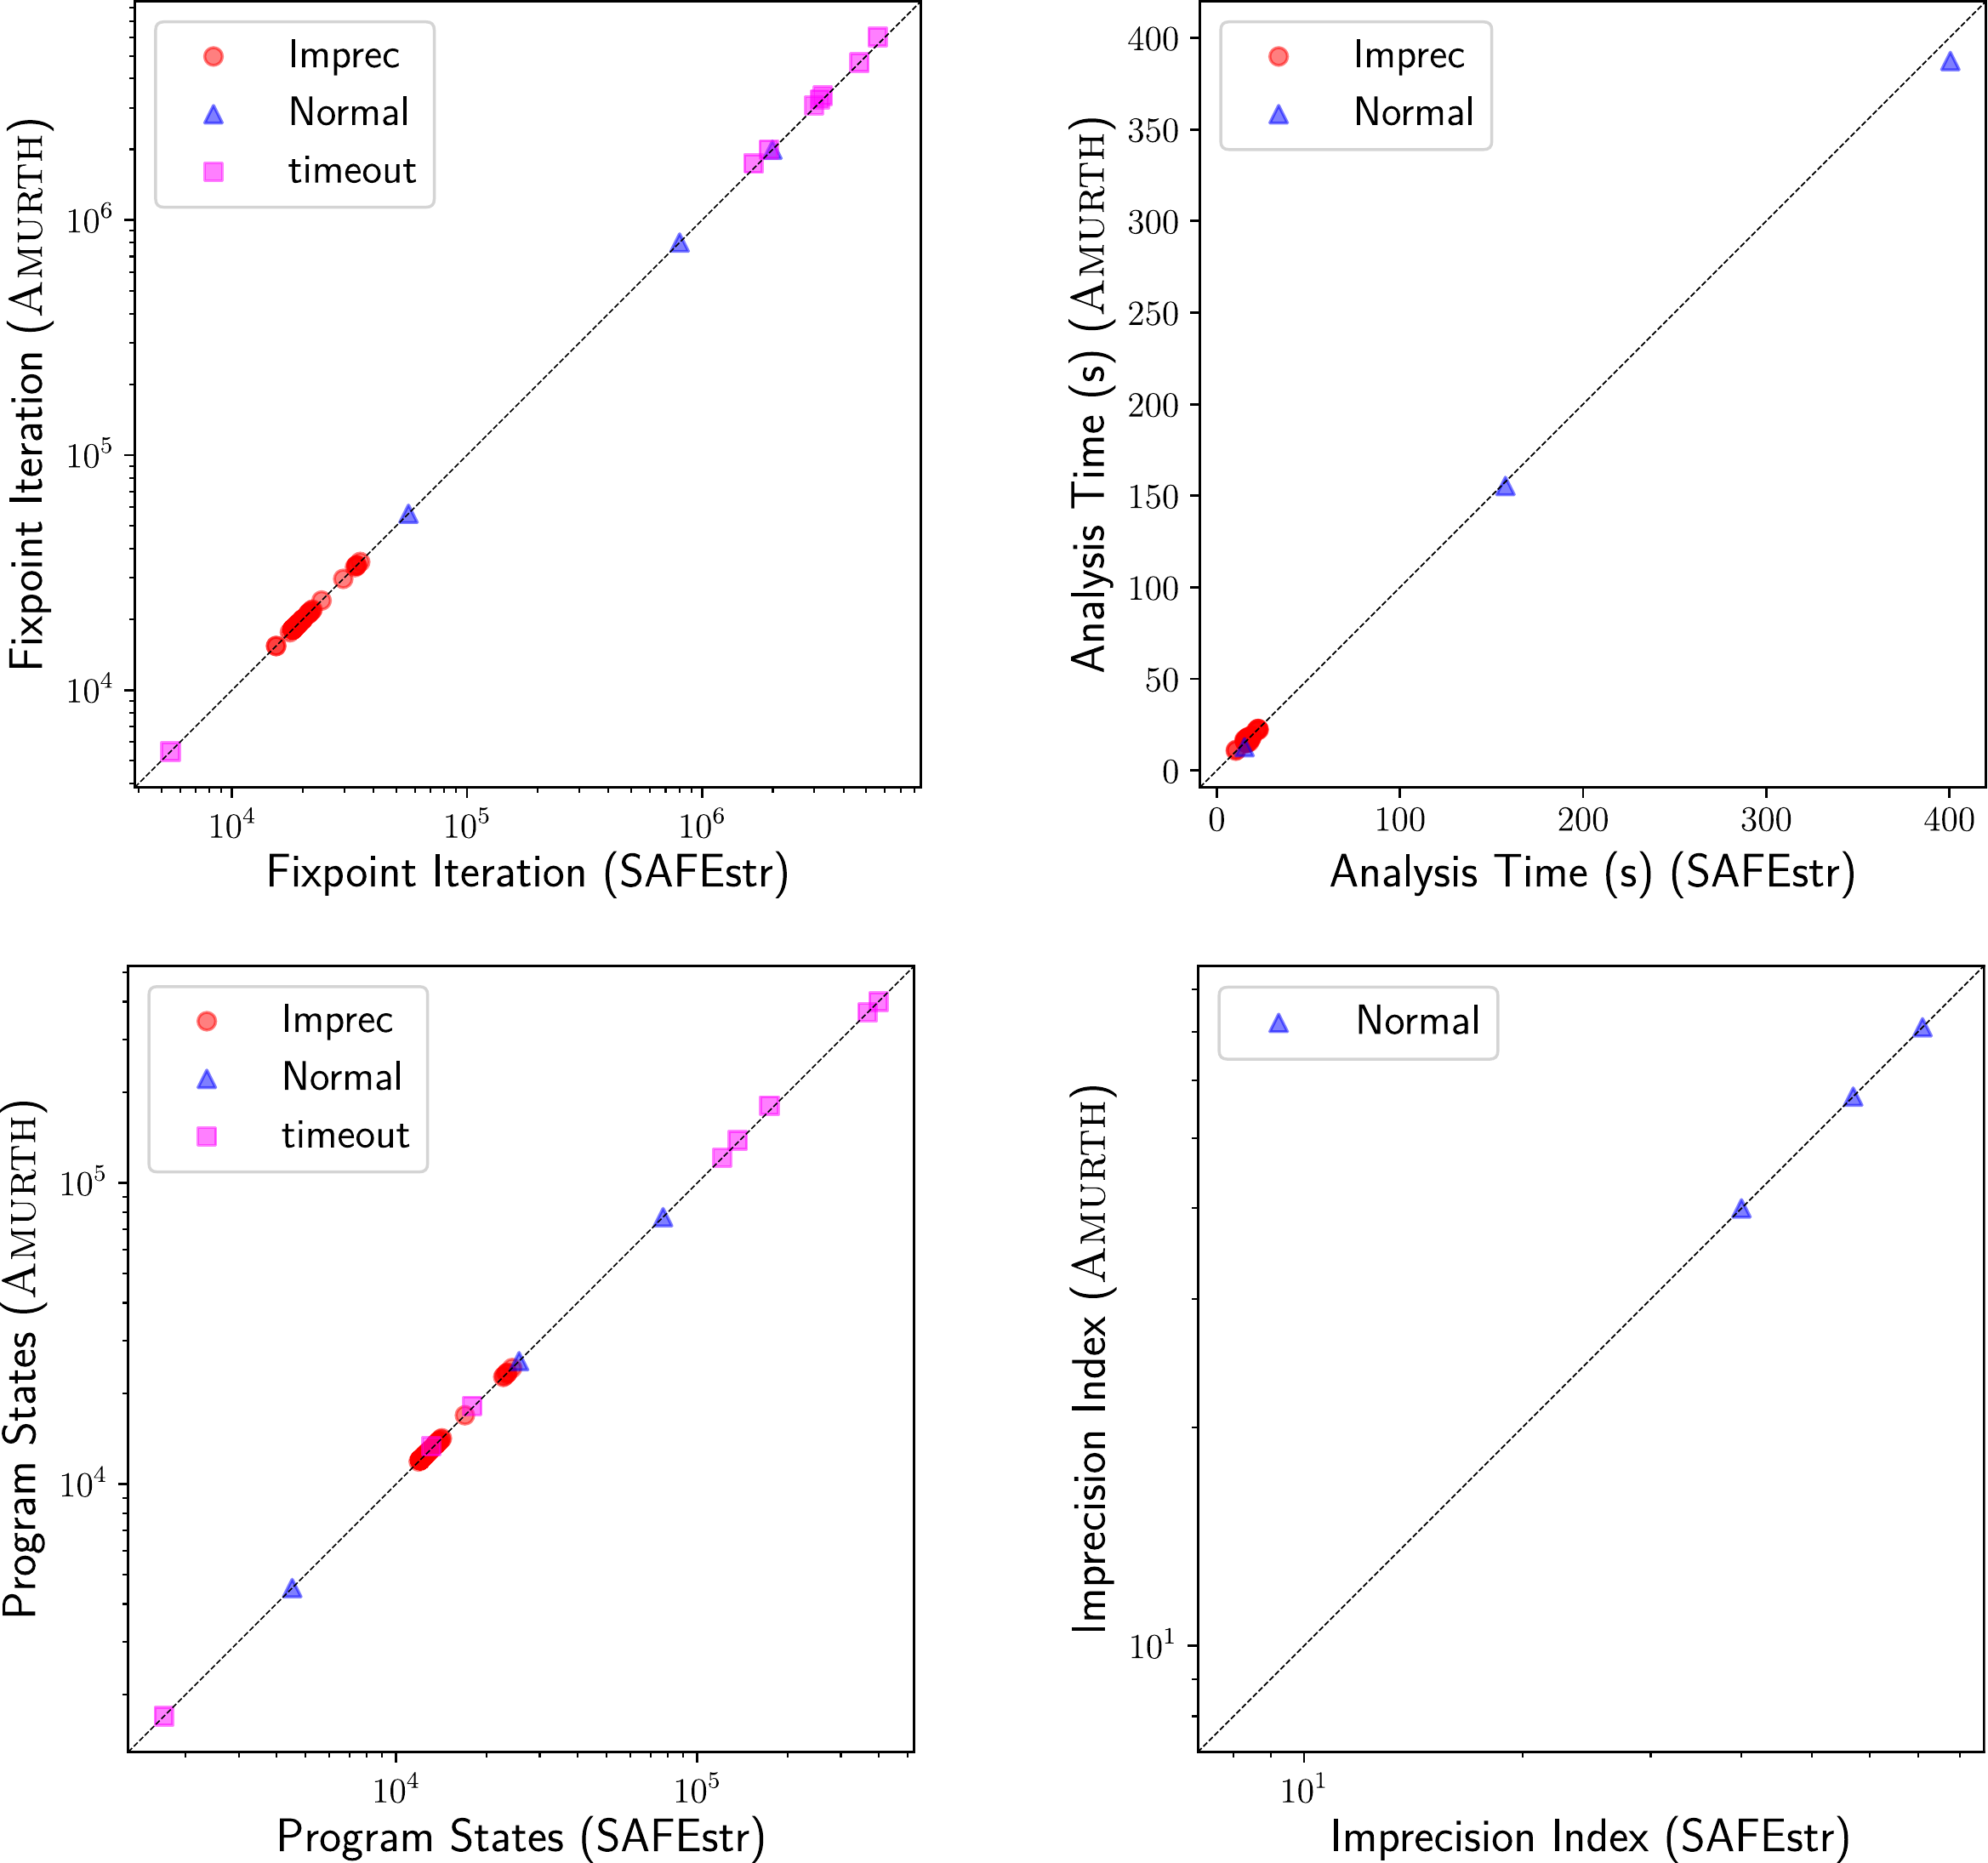}
	\caption{Performance and precision of the synthesized transformers  with the $\ssk$ domain $(k = 3)$.
		\label{Fi:SSKEvaluation}}
\end{figure}

\begin{figure}
	\centering
	\includegraphics[scale=0.35]{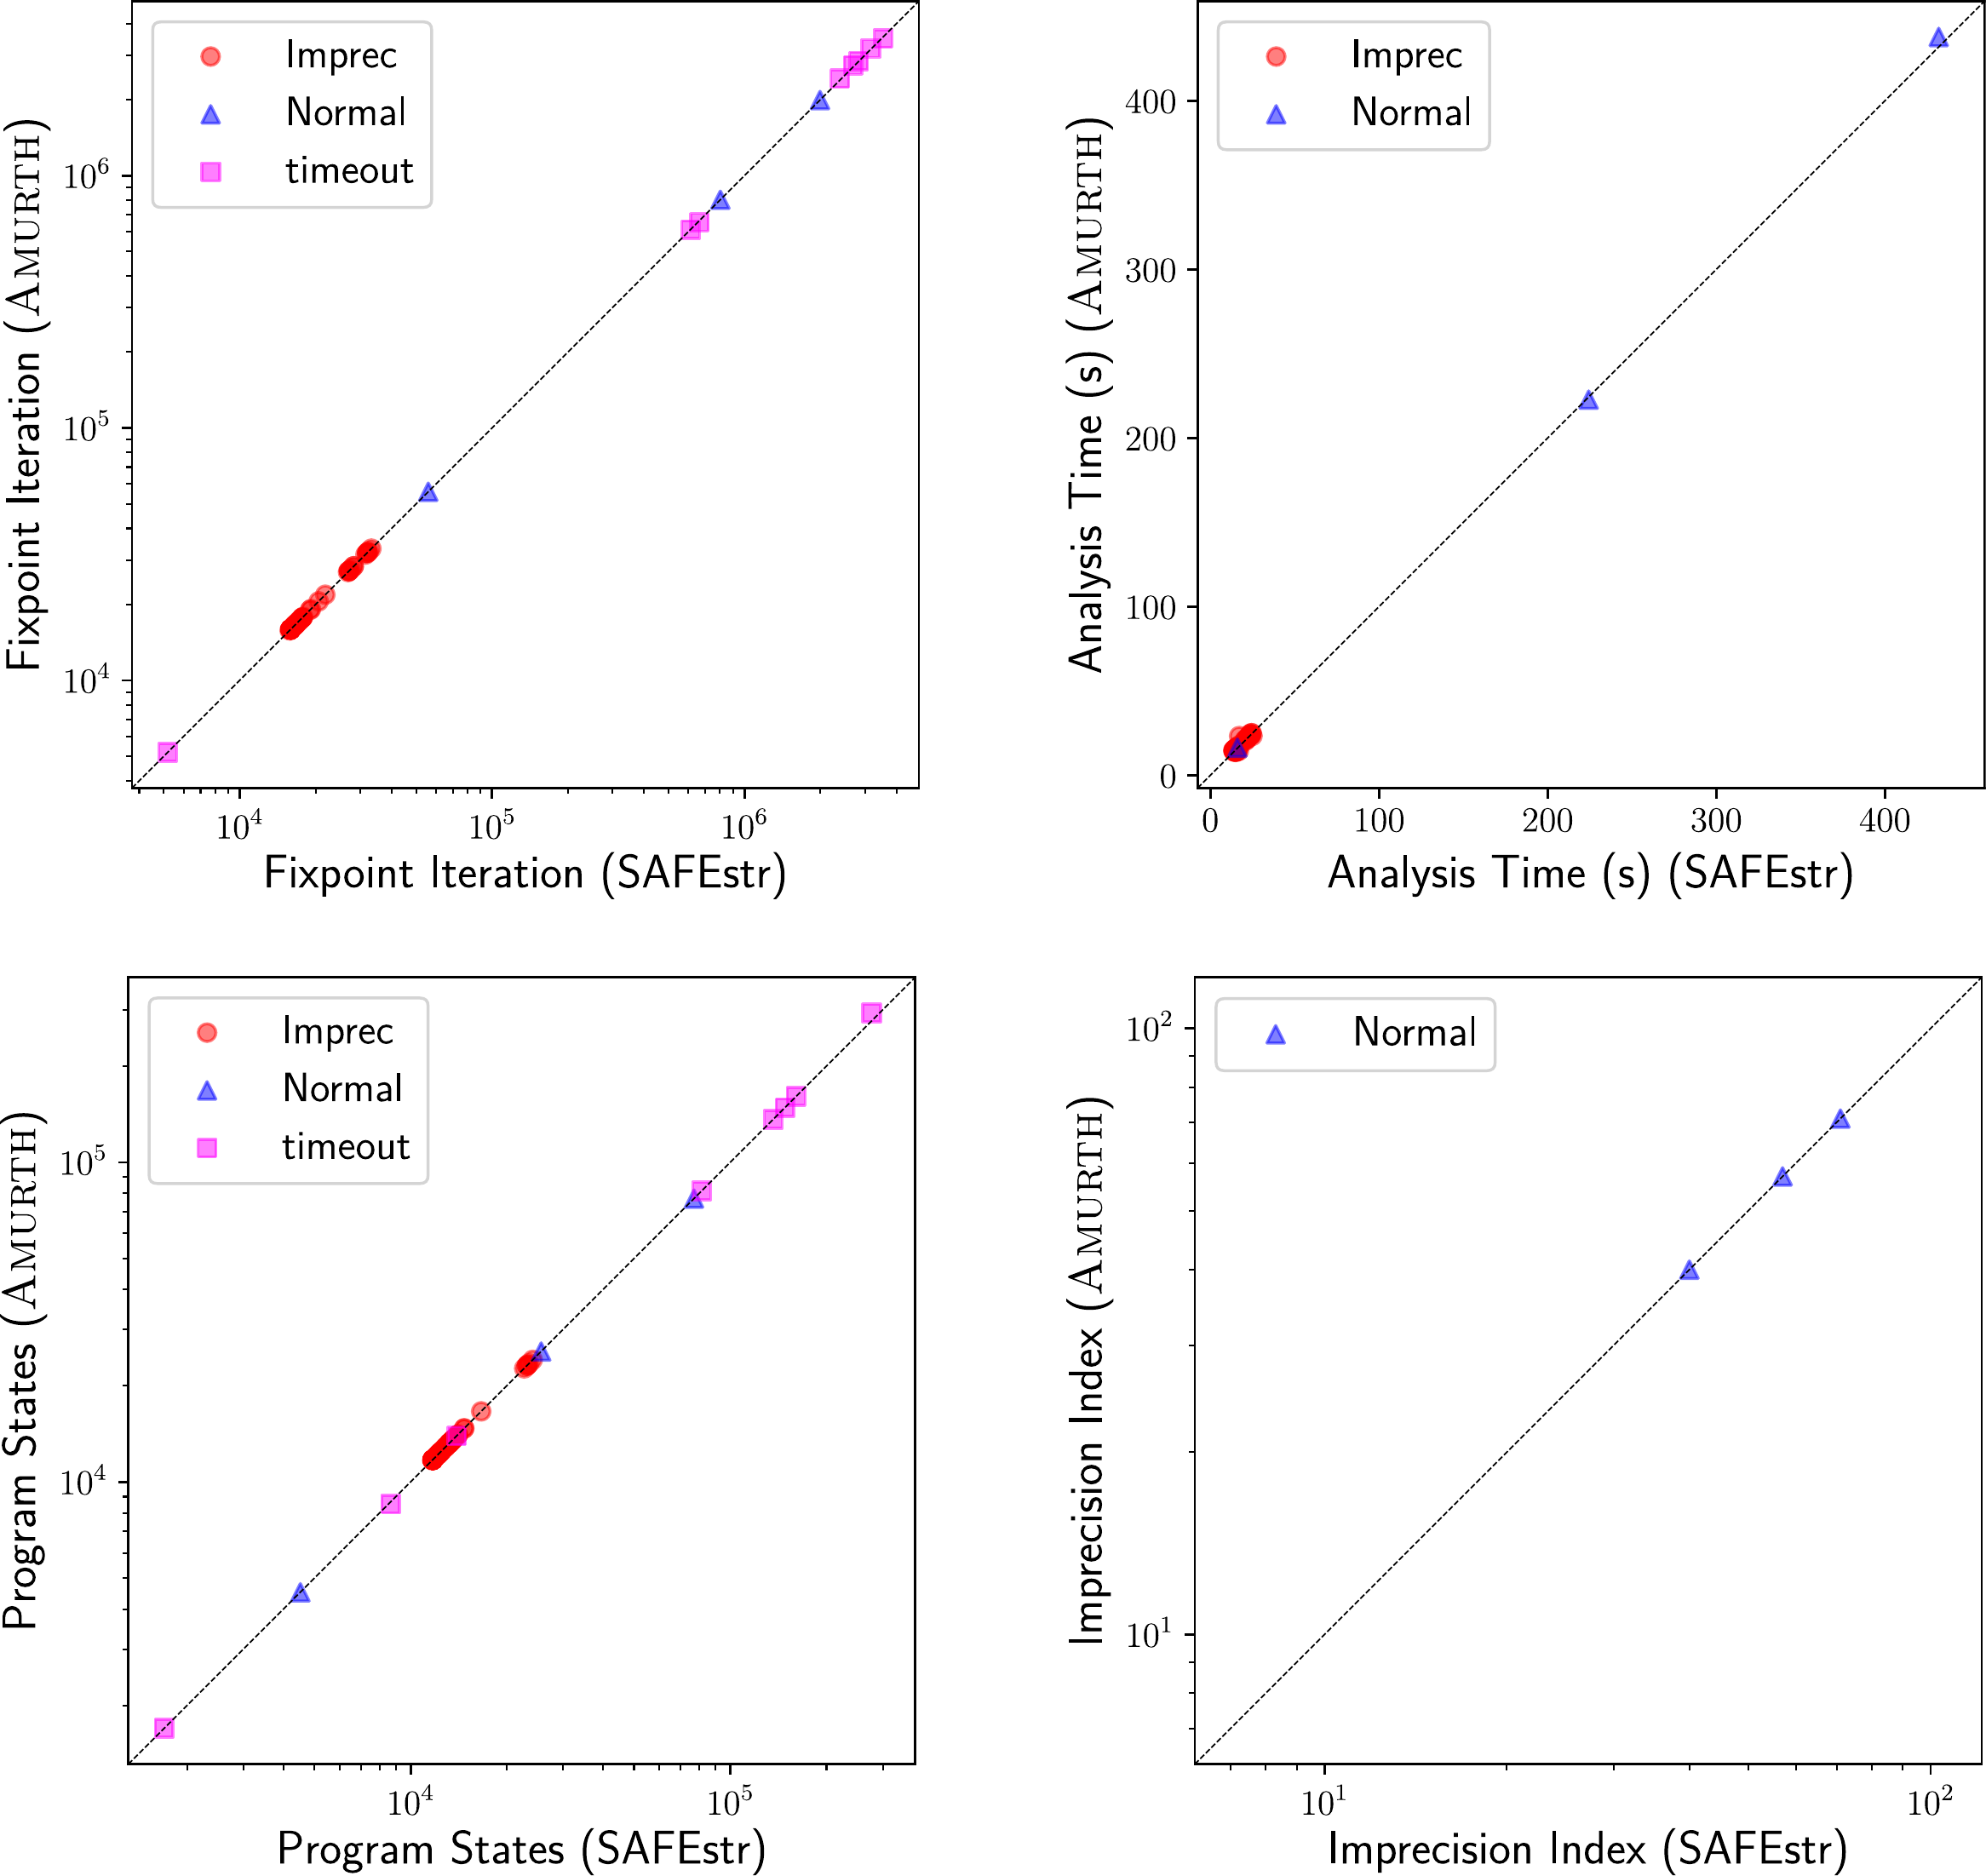}
	\caption{Performance and precision of the synthesized transformers with the product domain $\csdom \times \psdom$.
		\label{Fi:CoPsEvaluation}}
\end{figure}

\begin{table*}[t]
	\small
    \caption{Table showing detailed results for the string-domain experiments.\label{Ta:StringDomLogicalLog}}
%    \label{Ta:string-domain-detailed-logical-specifications}
    \begin{tabular}{|r|r|r|r|r|r|r|r|r|r|}
        \hline
        $f$ &\#SO&\#PO&\#PosEx&\#NegEx&\#MaxSat&\#Dropped&SO Time (s)&PO Time (s)&Time (s)\\ \hline \hline

        \multicolumn{10}{l|}{\cellcolor{black}\textcolor{white}{\textit{\textbf{$\mathcal{CS}$}}}}\\

        \texttt{charAt}		& 2 & 4 & 15 & 12 & 0 & 0 & 1.75 & 16.29 & 18.29\\ \hline
        \texttt{concat}		&2 & 16 & 19 & 16 & 0 & 0 & 2.03 & 96.26 & 99.05\\ \hline
        \texttt{contains}	&2 & 28 & 15 & 29 & 0 & 0 & 1.84 & 129.6 & 132.06\\ \hline
        \texttt{toLower}	&2 &6&7&12&0&0&1.74&9.19&11.26\\ \hline
        \texttt{toUpper}	&2 & 5 & 7 & 11 & 0 & 0 & 1.77 & 7.70 & 9.77\\ \hline
        \texttt{trim}		&2 & 2 & 11 & 0 & 0 & 0 & 1.81 & 2.40 & 4.31\\ \hline

        \multicolumn{10}{l|}{\cellcolor{black}\textcolor{white}{\textit{\textbf{$\mathcal{SS}_k$}}}}\\

        \texttt{charAt}		& 2 & 2 & 5 & 0 & 0 & 0 &1.89 & 1.90 & 3.94 \\ \hline
        \texttt{concat}		& 2 & 6 & 5 & 2 & 1 & 1 & 0.93 & 6.80 & 9.57 \\ \hline
        \texttt{contains} 	& 3 & 10 & 8 & 4 & 1 & 1 & 12.55 & 63.16 & 78.42 \\ \hline
        \texttt{toLower}	& 2 & 6 & 3 & 2 & 0 & 0 & 2.19 & 7.65 &11.74 \\ \hline
        \texttt{toUpper}	& 2 & 6 & 3 & 2 & 0 & 0 & 2.16 & 8.00 & 12.18 \\ \hline
        \texttt{trim}		& 2 & 6 & 3 & 2 & 0 & 0 & 1.93 & 12.74 & 16.35\\ \hline

        \multicolumn{10}{l|}{\cellcolor{black}\textcolor{white}{\textit{\textbf{$\mathcal{CI}$}}}}\\

        \texttt{charAt}		& 3 & 4 & 14 & 6 & 0 &0 & 5.46 & 13.25 & 24.91 \\ \hline
        \texttt{concat}		& 3 & 8 & 4 & 8 & 0 & 0 & 602.53 & 1,380.92 & 1,983.83\\ \hline
        \texttt{contains}   & 5 & 25 & 15 & 17 & 2 & 2 & 607.40 &  1,189.36 & 1,804.69 \\ \hline
        \texttt{toLower}	& 2 & 3 & 7 & 1 & 0 & 0 & 202.25 & 179.28 & 381.65\\ \hline
        \texttt{toUpper}	& 2 & 3 & 5 & 1 & 0 & 0 & 601.04 & 133.97 & 735.13 \\ \hline
        \texttt{trim}		& 5 & 24 & 10 & 12 & 0 & 0 & 11.75 & 624.89 & 641.53 \\ \hline

        \multicolumn{10}{l|}{\cellcolor{black}\textcolor{white}{\textit{\textbf{$\mathcal{PS}$}}}}\\

        \texttt{charAt}		& 2 & 5 & 13 & 3 & 0 & 0 & 1.81 & 3.95 & 5.94\\ \hline
        \texttt{concat}		& 2 & 5 & 3 & 7 & 0 & 0 & 0.59 & 8.20 & 8.92\\ \hline
        \texttt{contains}	& 3 & 8 & 2 & 2 & 1 & 1 & 2.27 & 5.41 & 9.13\\ \hline
        \texttt{toLower}	& 2 & 5 & 5 & 3 & 0 & 0 & 2.75 & 4.03 & 6.91\\ \hline
        \texttt{toUpper}	& 2 & 5 & 5 & 3 & 0 & 0 & 1.73 & 3.99 & 5.85\\ \hline
        \texttt{trim}		& 2 & 5 & 11 & 3 & 0 & 0 & 1.74 & 6.58 & 8.52\\ \hline

        \multicolumn{10}{l|}{\cellcolor{black}\textcolor{white}{\textit{\textbf{$\mathcal{SH}$}}}}\\

        \texttt{charAt}		& 2 & 2 & 7 & 0 & 0 & 0 & 1.84 & 1.78 & 3.76\\ \hline
        \texttt{concat}		& 2 & 2 & 9 & 0 & 0 & 0 & 600.89 &8.07 & 609.30\\ \hline
        \texttt{contains}	& 3 & 8 & 7 & 3 & 1 & 1 & 2.56 & 6.15 & 10.39\\ \hline
        \texttt{toLower}	& 4 & 6 & 3 & 0 & 0 & 0 & 2.99 & 5.29 & 8.44\\ \hline
        \texttt{toUpper}	& 2 & 2 & 1 & 0 & 0 & 0 & 1.87 & 1.75 & 3.73\\ \hline
        \texttt{trim}		& 4 & 6 & 3 & 0 & 0 & 0 & 2.82 & 5.29 & 8.29\\ \hline

    \end{tabular}
\end{table*}

\Omit{
\begin{table*}[htbp]
	 \small
    \caption{Table showing detailed results for the string-domain experiments with closed-box operations.\label{Ta:StringDomAFLLog}}
%    \label{Ta:string-domain-detailed-closed-box}
    \begin{tabular}{|r|r|r|r|r|r|r|r|r|r|}
    	
        \hline
        $f$ &\#SO&\#PO&\#PosEx&\#NegEx&\#MaxSat&\#Dropped&SO Time (s)&PO Time (s)&Time (s)\\ \hline \hline

        \multicolumn{10}{l|}{\cellcolor{black}\textcolor{white}{\textit{\textbf{$\mathcal{CS}$}}}}\\

        charAt&2&3&15&11&0&0&604.80&4.90&609.91 \\ \hline
        concat&2&13&19&13&0&0&604.61&31.49&636.38 \\ \hline
        contains&2&18&21&20&0&0&607.50&48.76&656.63 \\ \hline
        toLower&2&7&7&13&0&0&604.98&5.07&610.21 \\ \hline
        toUpper&2&5&7&11&0&0&604.54&4.26&608.93 \\ \hline
        trim&2&5&11&3&0&0&604.70&3.52&608.31 \\ \hline \hline

        \multicolumn{10}{l|}{\cellcolor{black}\textcolor{white}{\textit{\textbf{$\mathcal{SS}_k$}}}}\\

        charAt&2&6&5&2&0&0&605.33&4.49&611.35 \\ \hline
        concat&2&6&5&2&1&1&604.86&5.94&612.40 \\ \hline
        contains&6&32&13&18&5&7&692.09&57.95&758.97 \\ \hline
        toLower&2&6&3&2&0&0&605.13&6.45&613.28 \\ \hline
        toUpper&2&6&3&2&0&0&604.94&5.46&612.04 \\ \hline
        trim&2&6&3&2&0&0&604.86&9.64&617.24 \\ \hline \hline

        \multicolumn{10}{l|}{\cellcolor{black}\textcolor{white}{\textit{\textbf{$\mathcal{CI}$}}}}\\

        charAt&3&4&14&6&0&0&671.36&20.90&697.98 \\ \hline
        concat&2&5&3&7&0&0&606.49&672.84&1279.64 \\ \hline
        contains&10&56&29&28&7&13&1007.47&3183.73&4202.63 \\ \hline
        toLower&2&4&7&2&0&0&607.99&140.03&748.31 \\ \hline
        toUpper&2&5&11&5&1&1&605.76&5.58&615.96 \\ \hline
        trim&7&25&12&9&3&3&718.13&1824.55&2547.46 \\ \hline \hline

        \multicolumn{10}{l|}{\cellcolor{black}\textcolor{white}{\textit{\textbf{$\mathcal{PS}$}}}}\\

        charAt&5&28&16&16&2&3&623.02&25.41&652.91 \\ \hline
        concat&2&5&3&7&0&0&605.39&9.04&614.55 \\ \hline
        contains&3&8&2&2&1&1&609.51&5.32&616.26 \\ \hline
        toLower&2&2&5&0&0&0&604.70&1.95&606.74 \\ \hline
        toUpper&2&2&5&0&0&0&604.63&1.93&606.65 \\ \hline
        trim&2&5&5&6&0&0&604.78&10.53&615.66 \\ \hline \hline

        \multicolumn{10}{l|}{\cellcolor{black}\textcolor{white}{\textit{\textbf{$\mathcal{SH}$}}}}\\

        charAt&3&4&2&0&0&0&625.86&5.67&633.22 \\ \hline
        concat&2&2&1&0&0&0&605.08&2.52&607.84 \\ \hline
        contains&3&8&2&2&1&1&612.43&7.78&621.62 \\ \hline
        toLower&2&2&1&0&0&0&604.82&1.84&606.85 \\ \hline
        toUpper&2&5&1&1&1&1&605.85&5.51&616.91 \\ \hline
        trim&2&2&1&0&0&0&605.88&2.77&611.41 \\ \hline
    \end{tabular}

\end{table*}
}

\subsection{Fixed-Bitwidth Interval Domains}
\label{App:FixedBitwidthIntervalDomains}

%\fbox{\color{red}following section is intro to fixed-width interval domains as in Section~\ref{Se:casestudy1}, may be we can merge them}
\subsubsection{Abstract Transformers for Fixed-Bitwidth Interval Domains}
\label{App:IntervalDomsTransformers}
%In this study, we tried to synthesize abstract transformers for different operations shown in~\tableref{intervals-synthesis} for both signed- and unsigned-integer interval domains discussed in ~\cite{APLAS:WrInterval12}.

\Omit{
We used {\tool} to synthesize abstract transformers for nine operations for each of the three domains.
\tableref{intervals_synthesis} shows the time taken by {\tool} to synthesize each of the abstract transformers.
While in most cases, merely providing a DSL grammar was enough (indicated by the unshaded cells
in \tableref{intervals_synthesis}), for some of the more involved transformers, we had to provide
a sketch of the high-level implementation, and {\tool} was able to fill in the details (indicated by
the shaded cells).

All of the synthesized transformers are sound and precise, and are semantically equivalent to those
provided in the implementation that accompanies the \citeauthor{APLAS:WrInterval12} paper \cite{APLAS:WrInterval12}.
In one case, discussed in \sectref{absTransformXor},
when trying to synthesize a transformer while reusing some auxiliary
functions from the \citeauthor{APLAS:WrInterval12} implementation, we found that an
auxiliary function was implemented incorrectly---again underlining the
value of automatic synthesis of abstract transformers.
}

\tableref{IntvDomLogicSpecLog} shows the experimental results for
abstract-transformer synthesis in the fixed-bitwidth interval domains.

\begin{table*}[htbp]
    \caption{Table showing detailed results for the fixed-bitwidth interval-domain experiments. \textbf{\#MaxSat} and \textbf{\#Dropped} are 0 for all entries.\label{Ta:IntvDomLogicSpecLog}}
%    \label{Ta:interval-domain-detailed-logical-specifications}
    \begin{tabular}{|r|r|r|r|r|r|r|r|}
        \hline
        $f$ &\#SO&\#PO&\#PosEx&\#NegEx&SO Time (s)&PO Time (s)&Time (s)\\ \hline \hline
        \multicolumn{8}{l|}{\cellcolor{black}\textcolor{white}{\textit{\textbf{Unsigned}}}}\\
        \hline
        \texttt{add}	&2&7&11&25&1.79&130.28&133.70 \\
        \hline
        \texttt{sub}	&2&6&11&24&1.72&97.08&99.07 \\
        \hline
        \texttt{mul}		&2&35&3&33&10.78&1,434.62&1,449.85 \\
        \hline
        \texttt{and}		&2&5&7&3&1.80&12.56&14.54 \\
        \hline
        \texttt{or}		&2&4&0&2&1.82&15.39&17.36 \\
        \hline
        \texttt{xor}		&2&15&6&13&4.51&1,090.28&1,095.94 \\
        \hline
        \texttt{shl}	&2&5&7&5&1.81&10.51&12.52 \\
        \hline
        \texttt{ashr}	&2&3&1&7&1.82&4.16&6.15 \\
        \hline
        \texttt{lshr}	&2&5&3&7&2.89&9.79&12.88 \\
        \hline
        \multicolumn{8}{l|}{\cellcolor{black}\textcolor{white}{\textit{\textbf{Signed}}}}\\
        \hline
        \texttt{add}	&2&3&11&21&4.62&602.87&607.63 \\
        \hline
        \texttt{sub}	&2&8&11&26&11.03&200.60&213.17 \\
        \hline
        \texttt{mul}		&3&33&12&29&255.95&1,028.39&1,287.83 \\
        \hline
        \texttt{and}		&2& 3 & 17 & 1 & 130.15 & 153.98 & 284.42 \\
        \hline
        \texttt{or}		& 3 & 45 & 18 & 41 & 44.35 & 910.63 & 958.16 \\
        \hline
        \texttt{xor}		& 2 & 3 & 17 & 1 & 602.25 & 632.16 & 1,234.94 \\
        \hline
        \texttt{shl}	&2&4&3&4&1.90&9.43&11.78 \\
        \hline
        \texttt{ashr}	&2&4&5&6&1.94&5.49&7.61 \\
        \hline
        \texttt{lshr}	&2&2&3&4&1.84&2.07&4.23 \\
        \hline
        \multicolumn{8}{l|}{\cellcolor{black}\textcolor{white}{\textit{\textbf{Wrapped}}}}\\
        \hline
        \texttt{add}	&2&12&13&14&61.24&796.45&858.60 \\
        \hline
        \texttt{sub}	&2&12&13&14&14.46&724.19&739.47 \\
        \hline
        \texttt{mul}		&4 &12 &10 &8  &6.22 & 870.79& 880.12 \\
        \hline
        \texttt{and}		&2&5&5&3&623.38&737.12&1,360.98 \\
        \hline
        \texttt{or}		&2&5&5&3&621.31&689.64&1,311.37 \\
        \hline
        \texttt{xor}		&2&8&5&8&90.81&870.45&962.13 \\
        \hline
        \texttt{shl}	&2&7&19&5&11.71&186.53&198.90 \\
        \hline
        \texttt{ashr}	&2&8&7&10&450.54&147.31&598.62 \\
        \hline
        \texttt{lshr}	&4&19&9&19&276.20&270.80&548.72 \\
        \hline
    \end{tabular}
\end{table*}

\Omit{
\begin{table*}
    \caption{Table showing detailed results for the fixed-bitwidth interval-domain experiments with closed-box operations. \textbf{\#MaxSat} and \textbf{\#Dropped} are 0 for all entries.\label{Ta:IntvDomAFLLog}}
%    \label{Ta:interval-domain-detailed-closed-box}
    \begin{tabular}{|r|r|r|r|r|r|r|r|}
        \hline
        $f$ &\#SO&\#PO&\#PosEx&\#NegEx&SO Time (s)&PO Time (s)&Time (s)\\ \hline \hline
        \multicolumn{8}{l|}{\cellcolor{black}\textcolor{white}{\textit{\textbf{Unsigned}}}}\\
        \hline
        \texttt{add}	&2&6&11&24&607.48&131.76&739.68 \\ \hline
        \texttt{sub}	&2&11&1&9&604.96&6.28&611.55 \\ \hline
        \texttt{mul}		&2&24&11&22&613.35&2022.62&2639.38 \\ \hline
        \texttt{and}		&2&4&7&2&605.53&9.82&615.63 \\ \hline
        \texttt{or}		&2&5&7&3&605.53&12.09&617.93 \\ \hline
        \texttt{xor}		&2&13&5&11&665.34&721.42&1387.62 \\ \hline
        \texttt{shl}	&2&5&3&3&604.71&3.40&608.27 \\ \hline
        \texttt{ashr}	&2&3&7&7&605.87&4.30&610.39 \\ \hline
        \texttt{lshr}	&2&3&3&5&604.79&2.39&607.36 \\ \hline
        \multicolumn{8}{l|}{\cellcolor{black}\textcolor{white}{\textit{\textbf{Signed}}}}\\
        \hline
        \texttt{add}	&2&9&11&27&605.63&686.25&1292.35 \\ \hline
        \texttt{sub}	&2&6&11&24&605.84&157.41&763.56 \\ \hline
        \texttt{mul}		&3&34&12&30&621.26&488.19&1112.67 \\ \hline
        \texttt{and}		&2&3&17&1&605.87&411.17&1017.31 \\ \hline
        \texttt{or}		& 2 & 35 & 23 & 33 & 606.15 & 697.79 & 1306.37\\ \hline
        \texttt{xor}		&2&3&17&1&606.41&731.61&1338.29 \\ \hline
        \texttt{shl}	&2&5&3&5&606.25&8.77&615.36 \\ \hline
        \texttt{ashr}	&2&4&5&6&606.11&3.16&609.41 \\ \hline
        \texttt{lshr}	&3&6&4&6&620.27&9.65&630.27 \\ \hline
        \multicolumn{8}{l|}{\cellcolor{black}\textcolor{white}{\textit{\textbf{Wrapped}}}}\\ \hline
        \texttt{add}	& 2& 18& 13& 20& 605.30& 1252.58& 1858.71 \\ \hline
        \texttt{sub}	&2&15&13&17&607.49& 731.18 & 1339.34 \\ \hline
        \texttt{mul}	&4 & 9 & 10 & 5 & 1224.88 & 141.23 & 1368.57 \\ \hline
        \texttt{and}		&3&12&6&6&609.85&1691.29&2311.53 \\ \hline
        \texttt{or}		&2&6&5&4&605.08&750.33&1355.88 \\ \hline
        \texttt{xor}		&2&7&5&7&613.11&1134.33&1752.94 \\ \hline
        \texttt{shl}	&2&9&19&7&606.23&249.80&856.93 \\ \hline
        \texttt{ashr}	&2&12&3&14&605.21&89.05&694.86 \\ \hline
        \texttt{lshr}	& 3 & 22 & 8 & 22 & 621.36 & 376.02 & 1010.21 \\ \hline
    \end{tabular}
\end{table*}
}

%%% Local Variables:
%%% mode: latex
%%% TeX-master: "../main.tex"
%%% End:
